# Supplementary material for: Towards Robust and Automatic Hyper-Parameter Tunning
Source: arXiv:2111.14056 source file (2021-12-12)
Supplement: Supplementary file 1 [file main_supp.tex]

\documentclass[anon]{opt2021} % For LaTeX2e
\usepackage{times}

% Optional math commands from https://github.com/goodfeli/dlbook_notation.
\input{math_commands.tex}

\usepackage{hyperref}
\usepackage{url}
\usepackage{graphicx} %package to manage images
\usepackage{xcolor}
\usepackage{caption}
\captionsetup{format=plain} % % % % % %  here

\usepackage{mathtools}
\usepackage{amsmath}
\usepackage{physics}
\usepackage{comment}
\usepackage{siunitx}
\usepackage{algorithm}
\usepackage{algorithmic}
\usepackage{lscape}
\usepackage{multirow}
\usepackage{multicol}
\usepackage{pdflscape}
\usepackage{wrapfig}
\usepackage{soul}
\usepackage{pifont}% http://ctan.org/pkg/pifont

\graphicspath{ {./figures/} }
% \usepackage{algpseudocode}
% \algnewcommand{\algorithmicforeach}{\textbf{for each}}
% \algdef{SE}[FOR]{ForEach}{EndForEach}[1]
%   {\algorithmicforeach\ #1\ \algorithmicdo}% \ForEach{#1}
%   {\algorithmicend\ \algorithmicforeach}% \EndForEach
% \algrenewcommand\alglinenumber[1]{\scriptsize #1:}

% \DeclarePairedDelimiter\abs{\lvert}{\rvert}%
% \DeclarePairedDelimiter\floor{\lfloor}{\rfloor}

\makeatletter
\def\hlinewd#1{%
  \noalign{\ifnum0=`}\fi\hrule \@height #1 \futurelet
   \reserved@a\@xhline}

\definecolor{custom_green}{RGB}{40, 100, 219}
\definecolor{changed}{RGB}{0, 0, 0}
\definecolor{red}{RGB}{255, 100, 100}
\definecolor{green}{RGB}{40, 219, 100}
\definecolor{best}{RGB}{10, 150, 10}
\definecolor{close}{RGB}{255, 140, 0}
% \newcommand{\algorithmiccomment}[1]{\textcolor{custom_green}{\hskip1em // #1}}

% The \author macro works with any number of authors. There are two commands
% used to separate the names and addresses of multiple authors: \And and \AND.
%
% Using \And between authors leaves it to \LaTeX{} to determine where to break
% the lines. Using \AND forces a linebreak at that point. So, if \LaTeX{}
% puts 3 of 4 authors names on the first line, and the last on the second
% line, try using \AND instead of \And before the third author name.

\title{--Supplemental Material--\\Toward Robust and Automatic Tuning of Hyper-Parameters}

\begin{document}
\maketitle
\input{sections/appendix}
\clearpage
\bibliography{citations}

\end{document}
